# Supplementary material for: Unveiling the Reactivity of Oxygen and Ozone on C2N Monolayer: A First-Principles Study
Source: arXiv:2403.12454 source file (2024-03-19)
Supplement: Supplementary file 1 [file supporting_information.pdf]

## Supporting Information

# Unveiling the Reactivity of Oxygen and Ozone on $C_2N$ Monolayer: A First-Principles Study

Soumendra Kumar Das[1], Lokanath Patra[2], Prasanjit Samal[1*] and Pratap K. Sahoo[1*]

[1] *School of Physical Sciences, National Institute of Science Education and Research (NISER) Bhubaneswar, HBNI, Jatni, Khurda-752050, Odisha, India.*

[2]*Department of Mechanical Engineering, University of California, Santa Barbara, CA 93106, USA.*

*corresponding authors: E-mail: psamal@niser.ac.in, pratap.sahoo@niser.ac.in,

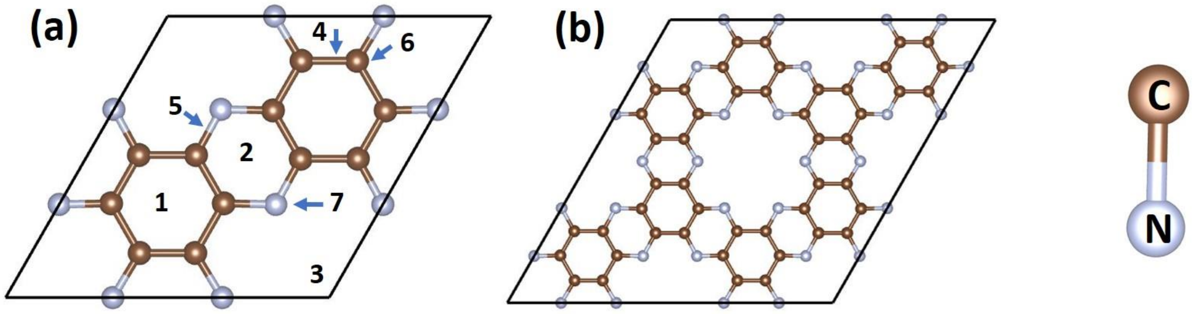


Figure S1: Schematic representation of pristine $C_2N$ monolayer with (a) $1 \times 1 \times 1$ and (b) $2 \times 2 \times 1$super cell configuration used for oxygen and ozone adsorption respectively. The 'C' and 'N' atoms are indicated by brown and grey colour respectively. The numbers given in S1(a) indicates the different locations on which the relax calculations were performed for oxygen and ozone adsorption at a distance of 4 Å from the surface. See Table S1, given below for details.

**Table S1:**

| Locations | Description |
|---|---|
| 1 | above benzine ring |
| 2 | above pyrazine ring |
| 3 | above hollow region |
| 4 | above C-C bond |
| 5 | above C-N bond |
| 6 | above 'C' atom |
| 7 | above 'N' atom |

**Table S2: Bond length and bond angle of oxygen and ozone molecules**

| Molecules | Bond length (Å) | | Bond angle (degree) | |
|---|---|---|---|---|
| oxygen | 1.24 | 1.24 (DFT)[1]<br>1.21 (Expt)[2] | | |
| ozone | 1.284 | 1.28 (Expt)[3]<br>1.28 (DFT)[4] | 118.23 | 116.74 (Expt)[3]<br>117.90 (DFT)[4] |

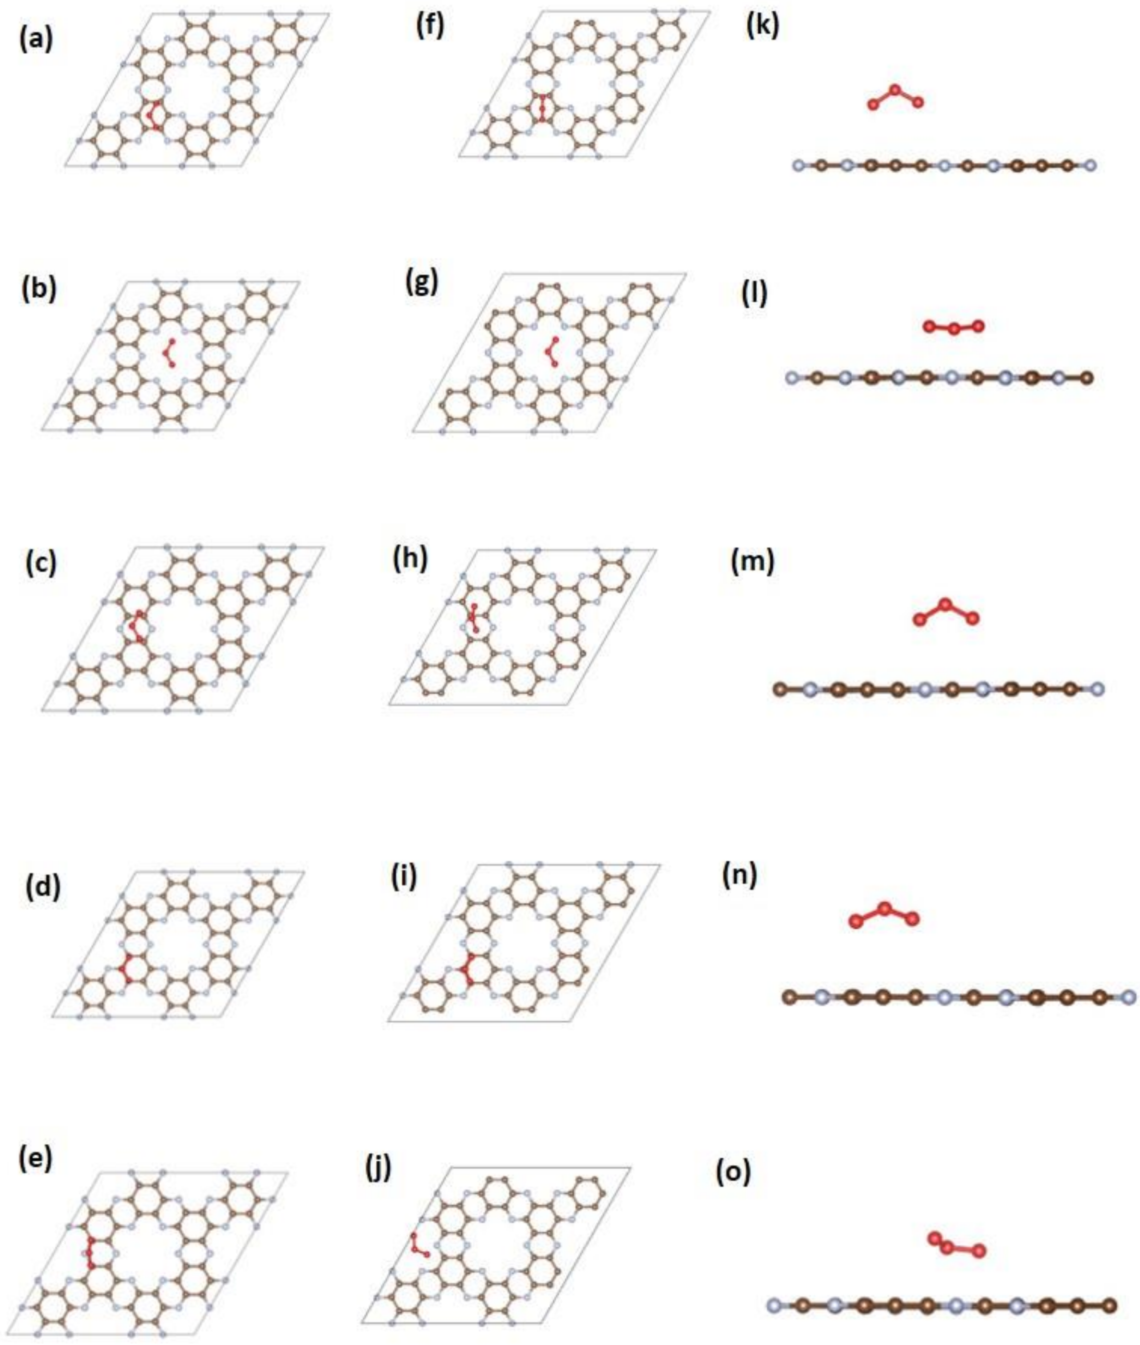


Figure S2: Geometrical optimization of ozone adsorbed $C_2N$ monolayer, The initial structure chosen for relax calculation where ozone molecule is placed **horizontally** at a distance 4 Å from $C_2N$ at different possible sites namely (a) inside benzene ring, (b) inside hollow region, (c) inside pyrazine ring, (d) on C-C bond, (e) on C-N bond. The corresponding structure after relax calculation are given in (e-i) for top view and (j-n) for side view.

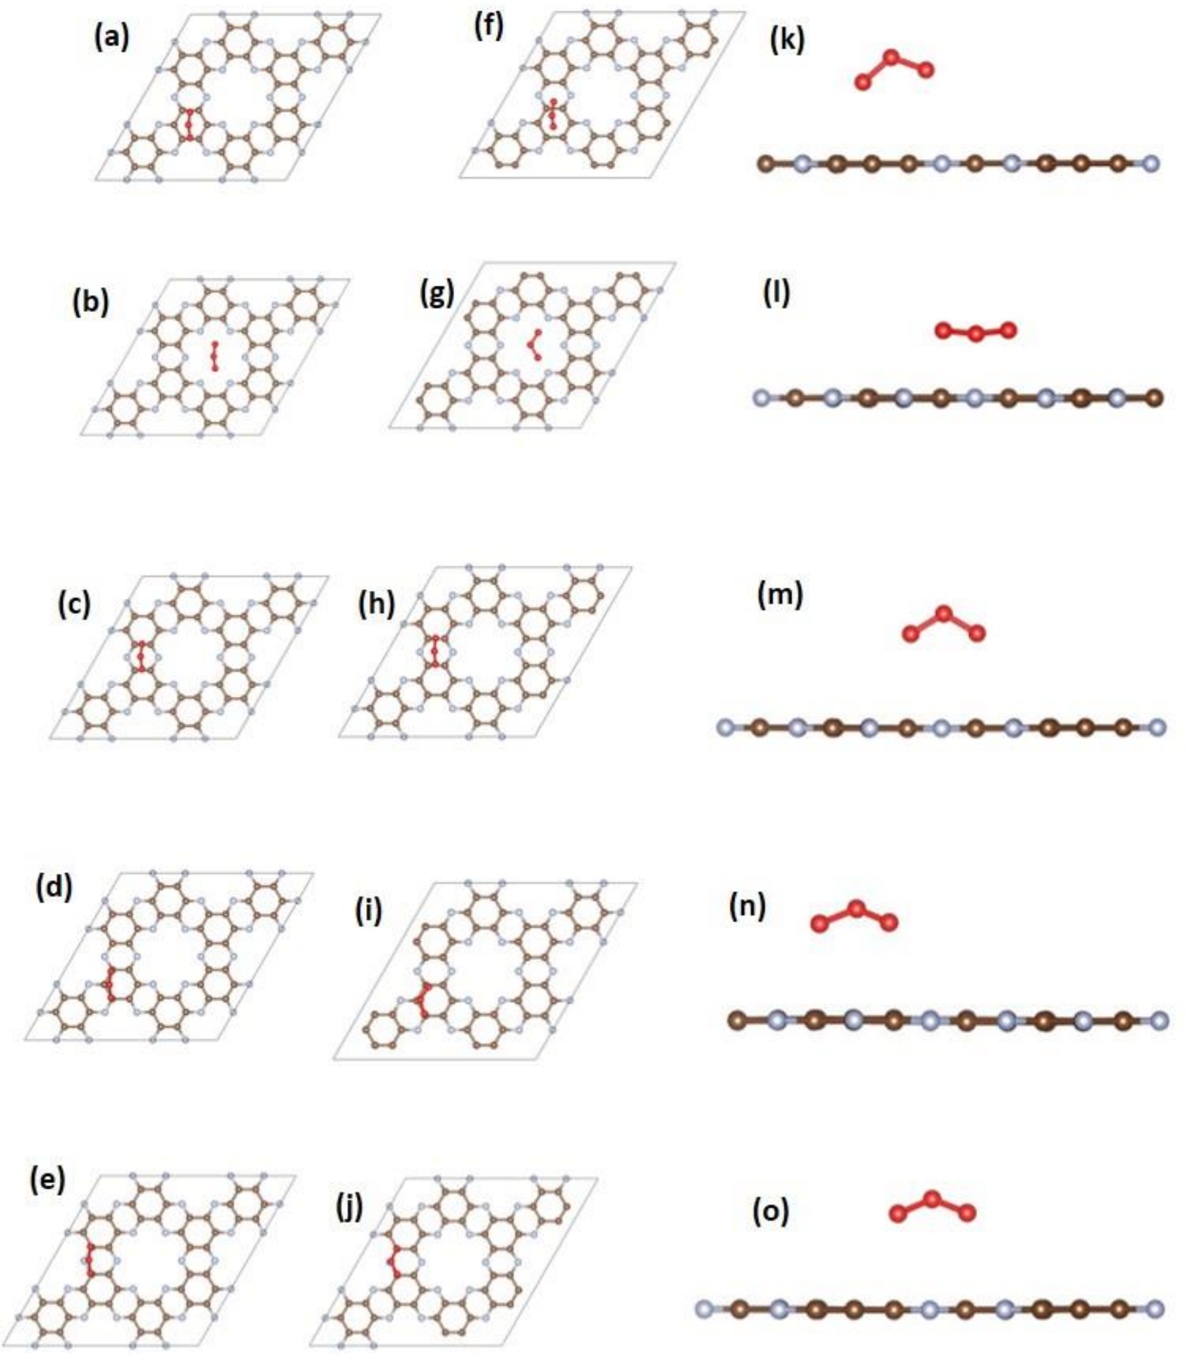


Figure S3: Geometrical optimization of ozone adsorbed $C_2N$ monolayer, The initial structure chosen for relax calculation where ozone molecule is placed **vertically with middle oxygen facing up** at a distance 4 Å from $C_2N$ at different possible sites namely (a) inside benzene ring, (b) inside hollow region, (c) inside pyrazine ring, (d) on C-C bond, (e) on C-N bond. The corresponding structure after relax calculation are given in (e-i) for top view and (j-n) for side view.

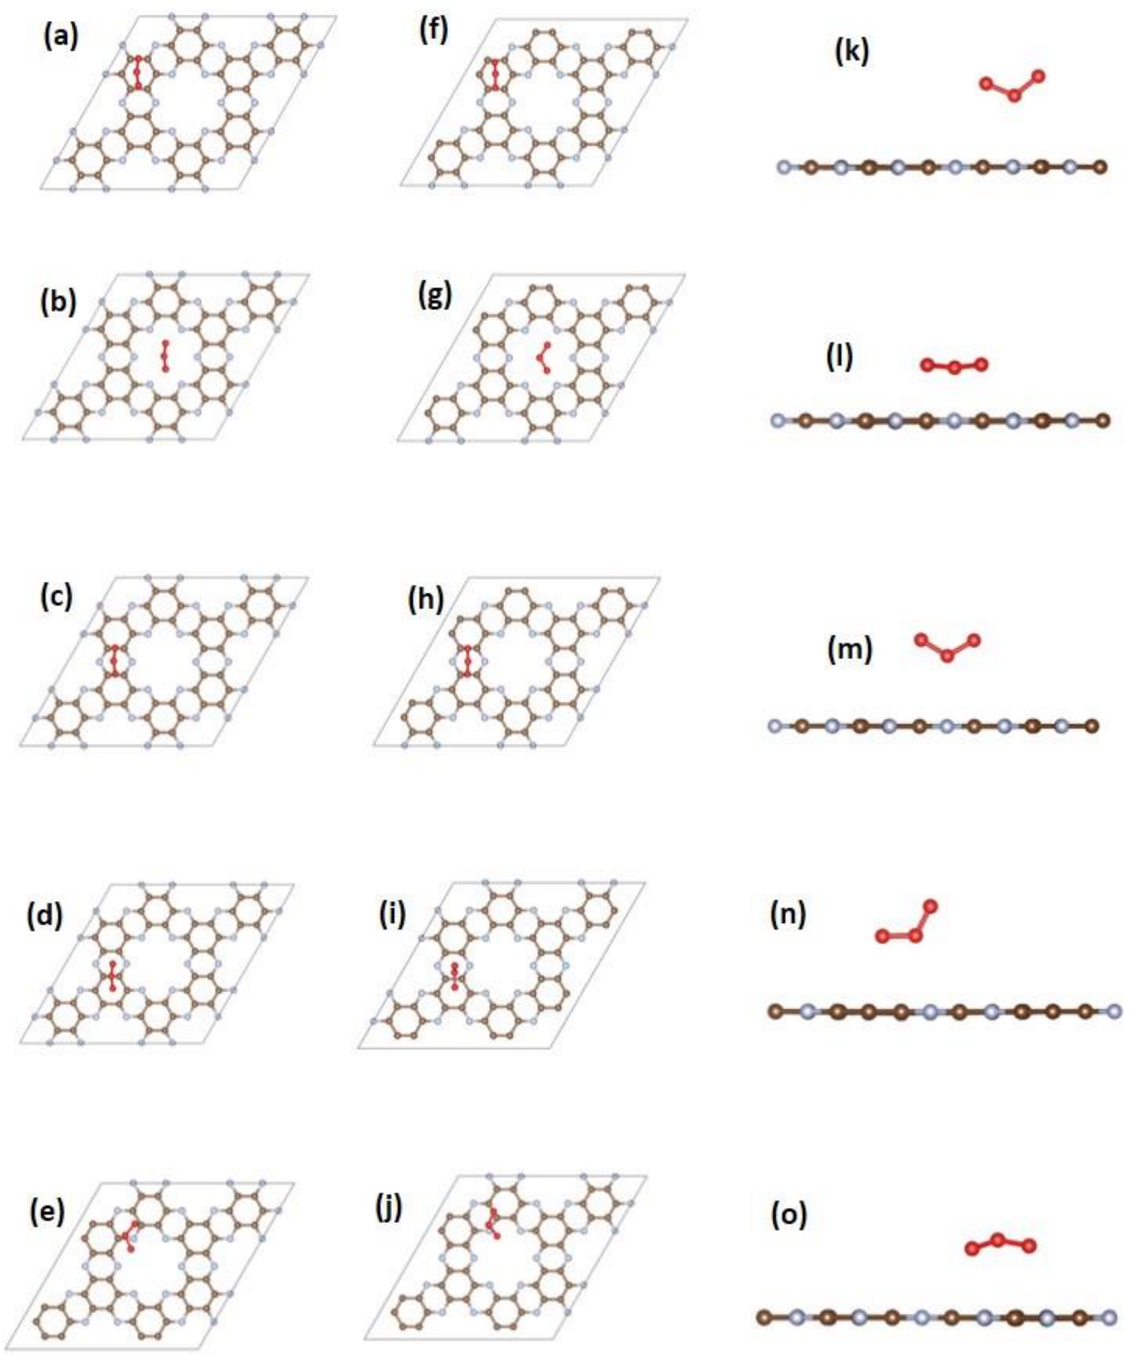


Figure S4: Geometrical optimization of ozone adsorbed $C_2N$ monolayer, The initial structure chosen for relax calculation where ozone molecule is placed **vertically with middle oxygen facing down** at a distance 4 Å from $C_2N$ at different possible sites namely (a) inside benzene ring, (b) inside hollow region, (c) inside pyrazine ring, (d) on C-C bond, (e) on C-N bond. The corresponding structure after relax calculation are given in (e-i) for top view and (j-n) for side view.

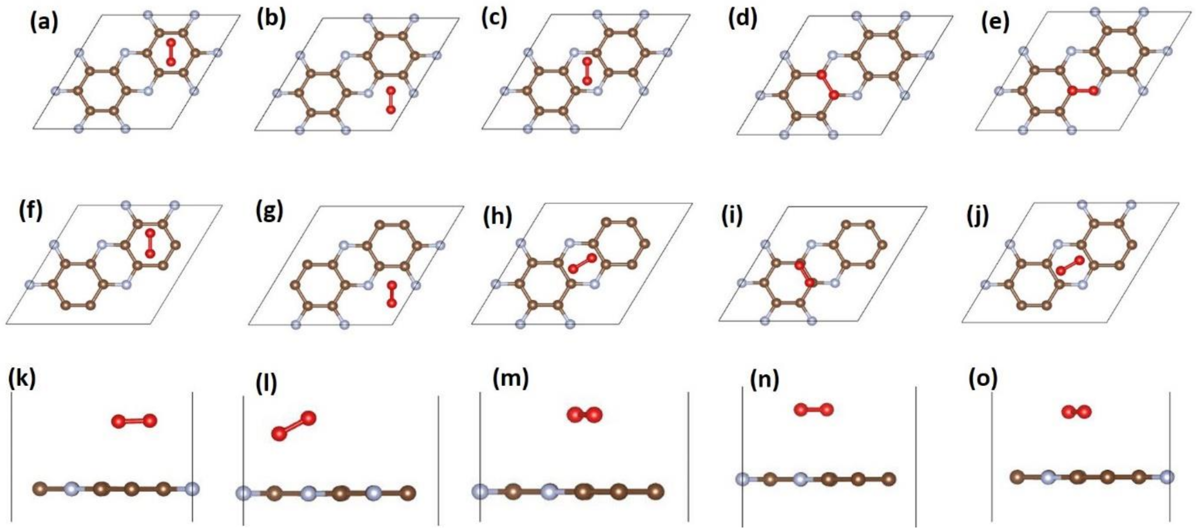


Figure S5: Geometrical optimization of oxygen adsorbed $C_2N$ monolayer, The initial structure chosen for relax calculation where oxygen molecule is placed **horizontally** at a distance 4 Å from $C_2N$ at different possible sites namely (a) inside benzene ring, (b) inside hollow region, (c) inside pyrazine ring, (d) on C-C bond, (e) on C-N bond. The corresponding structure after relax calculation are given in (f-j) for top view and (k-o) for side view.

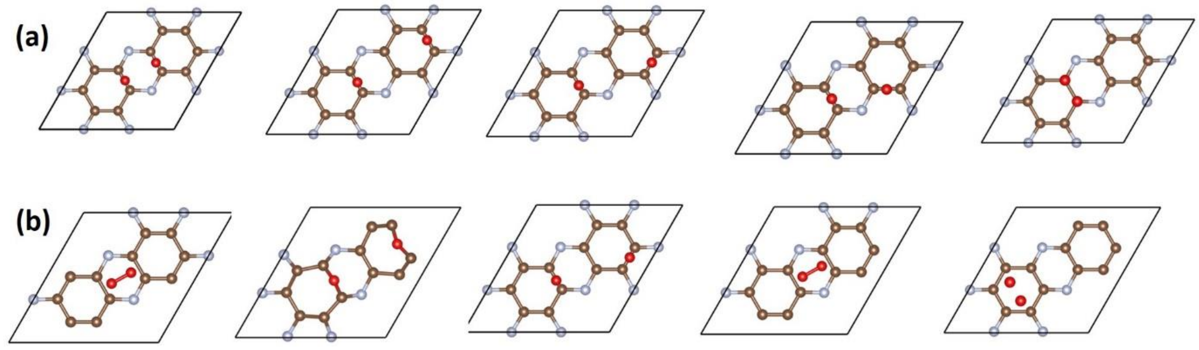


Figure S6: (Top Panel a) Geometrical optimization for atomic oxygen at different possible sites on $C_2N$ monolayer. The corresponding relaxed structures are given in the bottom Panel b.

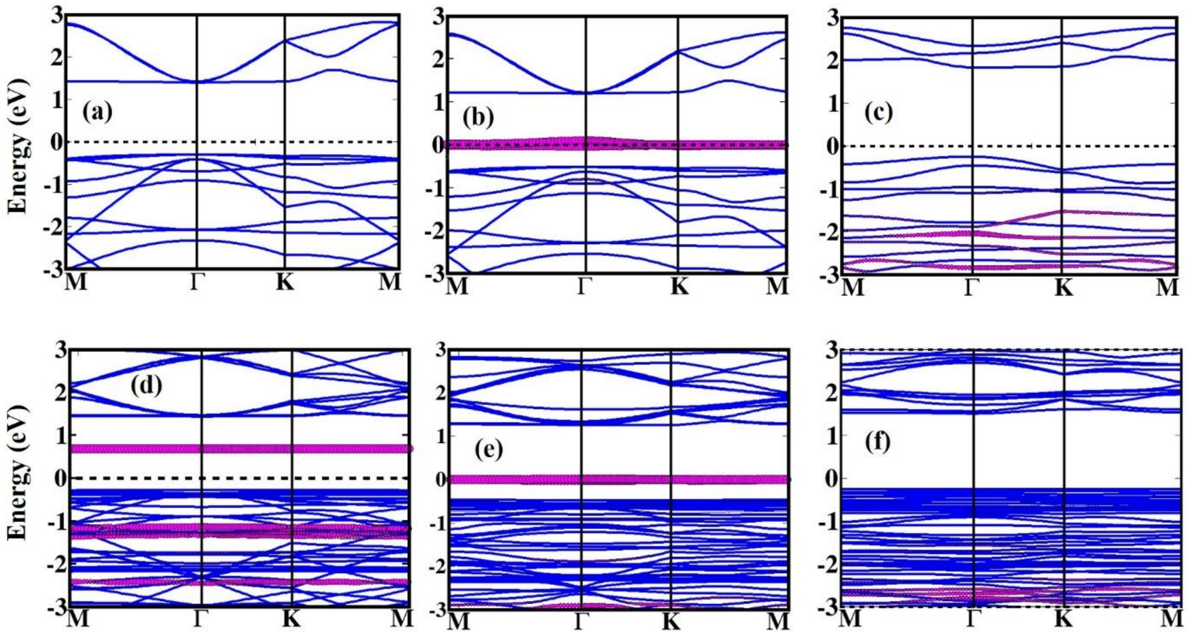


Figure S7: **Electronic structure of $O_2$/$O_3$ interaction with $C_2N$**. Top Panel: (a) Pristine $C_2N$, (b) Physisorbed ($O_2$) and (c) dissociated (O+O) oxygen configuration. Bottom panel: (d) physisorbed ($O_3$), (e) intermediate ($O_2$+O) and (f) dissociated (O+O+O) ozone configurations. The dotted horizontal line indicates the Fermi level.

## References

[1] A. Panchenko, M. Koper, T. Shubina, S. Mitchell, and E. J. J. o. t. E. S. Roduner, **151**, A2016 (2004).

[2] H. Nakatsuji and H. J. C. p. l. Nakai, **197**, 339 (1992).

[3] A. Kalemos and A. J. T. J. o. c. p. Mavridis, J. Chem. Phys. **129** (2008).

[4] D. Farmanzadeh and N. A. J. A. S. S. Ardehjani, Appl. Surf. Sci. **444**, 642 (2018).
